# Supplementary material for: Many-particle effects in the cyclotron resonance of encapsulated monolayer graphene
Source: arXiv:1709.00435 source file (2018-01-26)
Supplement: Supplementary file 1 [file interband_Supp_Matt.pdf]

## EXPERIMENTAL SETUP

Broadband infrared light from a Fourier-transform ir spectrometer is delivered to the sample via light pipe optics as shown schematically in Fig. S1. Light is focused to, and then defocused from, the sample using parabolic cone optics and finally gathered by a compound parabolic collector for detection at a composite Si bolometer held at 4 K. The sample, comprising a 40-nm-thick boron nitride–graphene–boron nitride stack with edge contacts [1], sits on an oxidized Si wafer; the lightly-doped Si serves as a back gate for the applied gate voltage. The infrared beam spot size is less than half a millimeter in diameter. The beam enters the bottom of the wafer, passes through and out the top side, uniformly illuminating the sample and much of the surrounding surface; and is stopped down by a $\approx 60$ $\mu$m aperture made of a small hole poked in Al foil. Thus much of the light detected at the bolometer has *not* passed through the graphene. We note the region around the contacts may become highly doped [2], but this region extends only $0.2 - 0.3$ $\mu$m into the sample; here, that amounts to less than 3% of the total device area. Moreover in these highly doped regions interband transitions in the energy range of interest will be blocked, so this effect does not impact our results.

## FITTING

Infrared magneto-spectroscopy was studied in a heterostructure device comprising five layers: a 620 $\mu$m thick, lightly doped silicon wafer; a 300 nm thermal oxide on the wafer surface; a thin crystal of hexagonal boron nitride (hbn) estimated to be 15 nm thick; a monolayer of graphene; and a top layer of hbn estimated to be 30 nm thick. Due to multiple reflections at the interfaces of different layers and the presence of multiple absorbing materials, transmission through such a stratified system is an involved function of the layer thicknesses and complex indices of refraction.

Multiple reflections within the stack produce frequency-dependent distortions of the Lorentzian line shape of Landau level transitions in the graphene monolayer. The observed resonances therefore appear asymmetric, with the spectral weight and central peak shifted from their actual values, preventing simple extraction of resonance energies and linewidths. To account for these distortions we performed a nonlinear fitting procedure using a model for transmission through a multilayer thin-film system [3, 4].

Constructing the multilayer reflection model requires accurate determination of the complex index of refraction $\tilde{n} = n + ik$ for each layer. For the Si/$SiO_2$ substrate this was accomplished via careful measurements of a piece of the same silicon wafer used in fabricating the device, both before and after removing the oxide layer. Standard fitting procedures employing the Reffit software package were then used to construct a model of the Si and $SiO_2$ complex indices of refraction [5]. For hexagonal boron nitride, values of $n$=1.8 and $k$=0 were assumed for all frequencies [6].

The dielectric function of the graphene monolayer was modeled as a set of Drude-Lorentz oscillators corresponding to

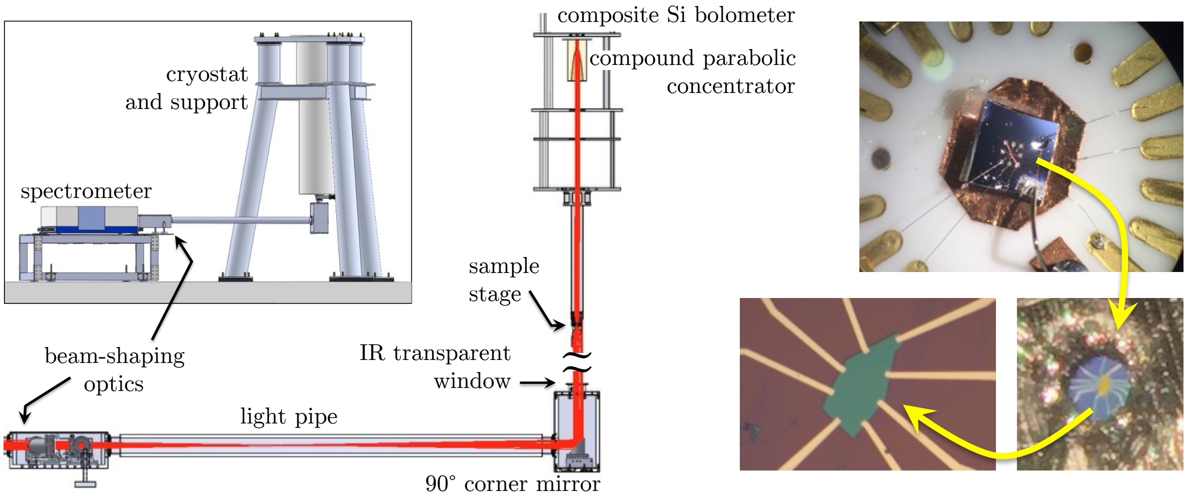


FIG. S1. Left: schematic of experimental setup showing light-pipe optics guiding infrared light from FTIR spectrometer to sample in cryostat and ultimately a composite Si bolometer. Right: progressively zoomed-in view of graphene/hbn stack on oxidized Si wafer, final beam stop via a hole in Al foil, and the device itself.

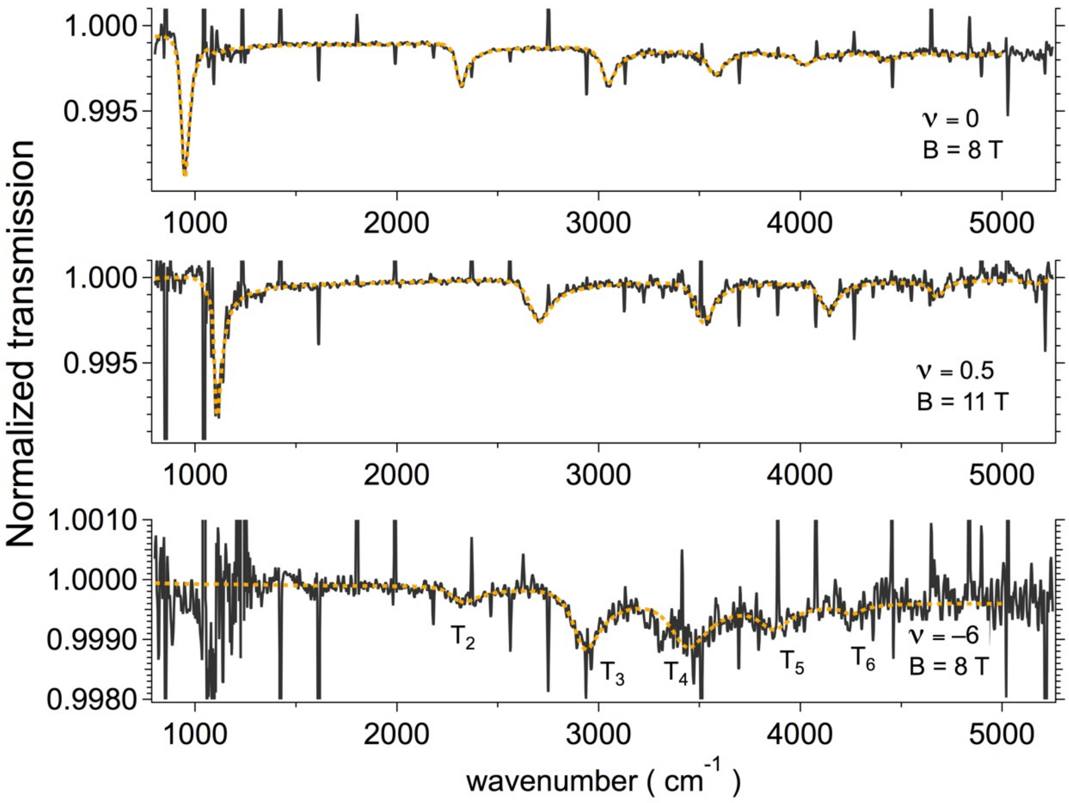


FIG. S2. Normalized infrared magneto-spectroscopy data plotted as $S(\nu)/S(\nu = 22)$, showing representative fits to several cyclotron resonance transitions in traces having (a) high, (b) moderate, and (c) low signal-to-noise ratios. For the fits in (c), error bars for the energies of the three highest energy resonances are taken to be the width of the transitions.

distinct Landau level transitions. Each Lorentzian is characterized by three parameters: a center frequency, a plasma frequency, and a linewidth. These parameters were allowed to vary until good agreement was achieved between the model and data, as determined by a quasi-Newton algorithm and checked by eye (see Fig. S2). In most cases, error bars for center frequencies are taken as the standard errors computed by the fitting procedure. For certain data traces where low signal-to-noise ratios prevented unambiguous determination of the center frequency (see Fig. S2c), error bars are taken as the width of the resonance.

## TRANSMISSION AT $B$=5 AND 11 T

Figure S3 shows the effective Fermi velocity $v_F^{ee}$ extracted from fits to the six observed transitions at two additional magnetic fields, $B$=5 and 11 T. Qualitatively, these data show the same behavior as the 8 T data in the main text: the values of $v_F^{ee}$ decrease with increasing filling factor and the specific dependences change with transition number. The 5 T data appear more rounded, likely due to the increased role of disorder as the LL separations shrink with decreasing magnetic field; and the 11 T data show concomitantly sharper plateaus at $|\nu|<2$ for the higher transitions. We note at 11 T the $T_1$ transition overlaps with a strong absorption feature in the substrate which greatly reduces our ability to extract the resonance energies.

The strongest feature in these data is the clear correlation of $v_F^{ee}$ with magnetic field: with increasing field, the average values of $v_F^{ee}$ decrease across the board. This "running of the velocity" with magnetic field has been predicted [8] and recently observed via magneto-Raman spectroscopy of graphene [9]. It is a consequence of the QED-like structure of the graphene dispersion [10].

As in Fig. 4 of the main text, we include predictions for $v_F^{ee}$ calculated using the many-particle theory of Ref. [7] for transitions $T_2$ and $T_3$. Again, only the rough contours of the data are captured by these calculations, and for $B$=5 T especially, there is a fair discrepancy in the absolute value of $v_F^{ee}$.

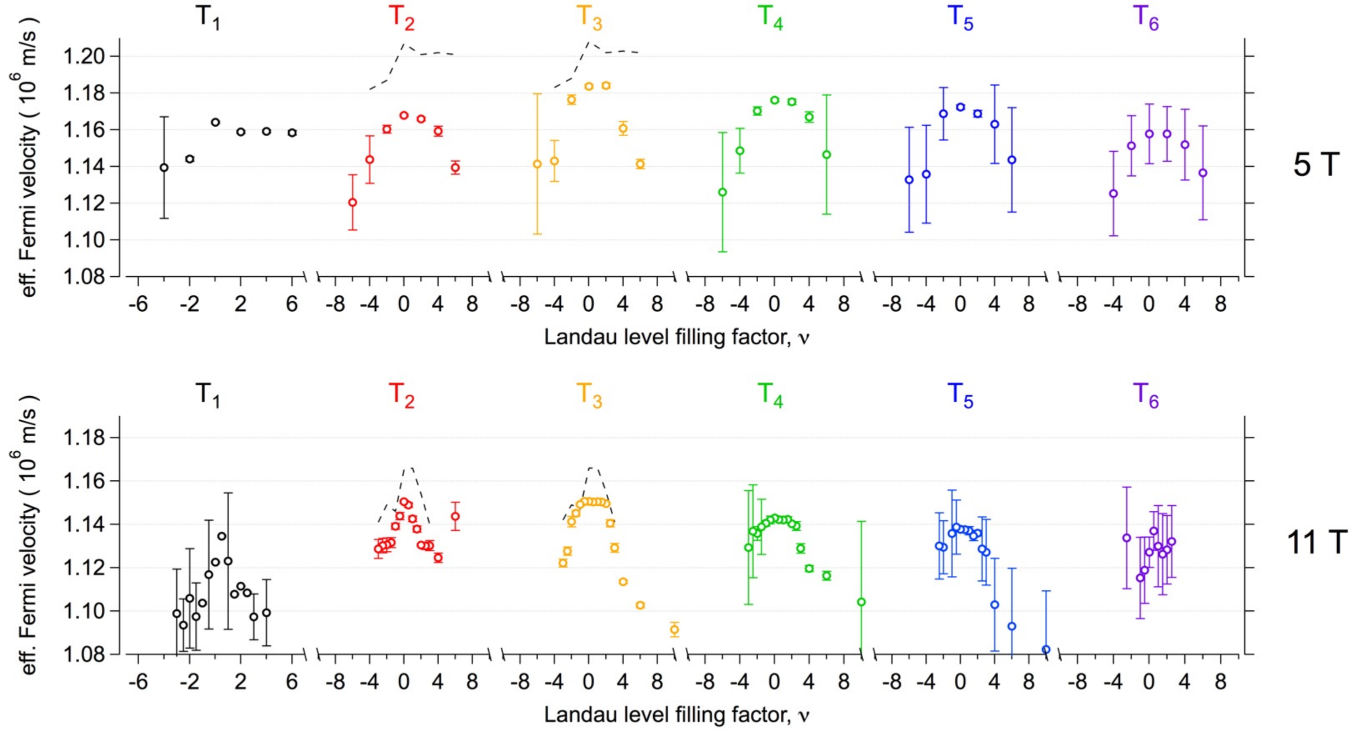


FIG. S3. Effective Fermi velocity at $B$=5 and 11 T for all six transitions as a function of filling factor, $\nu$=$nh/eB$. The black dashed lines in $T_2$ and $T_3$ are calculated from the theory of Ref. [7].

## $v_F^{ee}$ VS. TRANSITION NUMBER

In Fig. S4 and S5 we re-plot the aggregated $v_F^{ee}$ data from the main text and Fig. S3 as $v_F^{ee}$ vs. transition number, with one plot for each of several values of the filling factor, $\nu$=$0, \pm 2, \pm 4$, and $\pm 6$. Plotted this way, two features become immediately apparent: first as already noted, $v_F^{ee}$ of nearly every transition decreases for increasing magnetic field. Second, $v_F^{ee}$ varies with the transition number at each fixed filling factor, and the specific form of the variation evolves with changing $\nu$. For $\nu$=0 and $\pm 2$, $v_F^{ee}$ peaks at $T_3$. At higher $\nu$ values, however, the peak shifts to lower transition number. The overall variations can be succinctly, if qualitatively, captured by the diagram in Fig. 5 of the main text. There we construct schematic graphene dispersions by changing the slope of the usual Dirac cone to mimic the variations of $v_F^{ee}$ apparent in Fig. S4 and S5. This gives a qualitative picture of how $v_F^{ee}$ varies for transitions at higher energies, and as the Fermi level is moved through the LL structure.

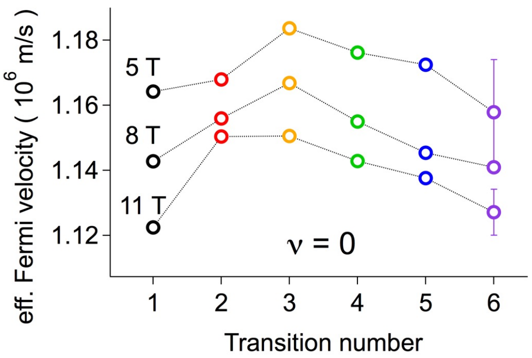


FIG. S4. $v_F^{ee}$ values for $\nu$=0, shown for all three fields, replotted vs. transition number; symbol colors match Fig. S3.

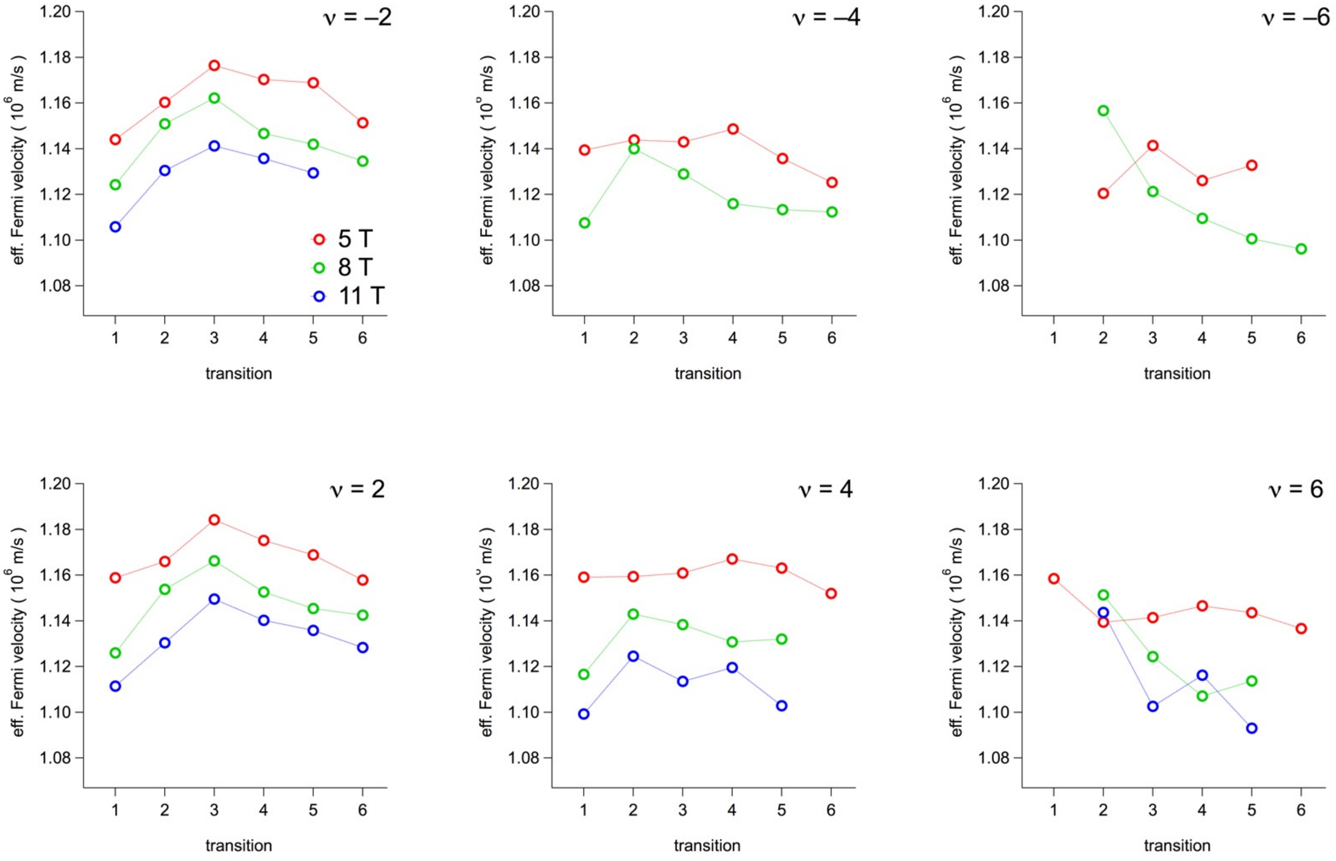


FIG. S5. $v_F^{ee}$ values at additional filling factors beyond just $\nu$=0, shown for all three fields, replotted vs. transition number. $B$=5, 8, and 11 T data shown in red, green, and blue, respectively.

## LANDAU LEVEL ENERGIES WHEN $N$=0 IS GAPPED

The presence of a gap in the $N$=0 level when $\nu = \pm 2$ is inferred by the splitting seen in $T_1$ (ascribed to sublattice symmetry breaking by the graphene/hbn coupling). Separately, the blueshift of $T_1$ at $\nu$=0 indicates the presence of an interaction-induced gap at half-filling of the $N$=0 level [4] (this gap arises in graphene even without the presence of boron nitride). Analyzed along the lines of Ref. [4], we infer the interaction-induced gap size to be ≈6 meV. A gap in the $N$=0 level will shift the energies of higher-index Landau levels according to [11]

$$E_n = \sqrt{2e\hbar v_F^2 Bn + (\Delta/2)^2} \ ,$$

with $n$ the LL index and $\Delta$ the gap size. Even for the larger 6 meV gap, this implies the energy of the $N$=1 LL is shifted by less than 0.05%. Since the $\nu$=0 gap is expected to close at other filling factors, a *very* small portion of observed decreased in $v_F^{ee}$ may be attributed to this effect. However the variations reported in Fig. 4 of the main text are of order a few %, far larger than the gap-induced shift, and thus in the main text we do not account for the shift of the LL energy due to gaps in the $N$=0 level.

[1] L. Wang, I. Meric, P. Y. Huang, Q. Gao, Y. Gao, H. Tran, T. Taniguchi, K. Watanabe, L. M. Campos, D. A. Muller, J. Guo, P. Kim, J. Hone, K. L. Shepard, and C. R. Dean, Science **342**, 614 (2013).
[2] T. Mueller, F. Xia, M. Freitag, J. Tsang, and P. Avouris, Physical Review B **79**, 245430 (2009).
[3] P. Yeh, *Optical Waves in Layered Media*, Wiley Series in Pure and Applied Optics (Wiley, 2005).
[4] E. A. Henriksen, P. Cadden-Zimansky, Z. Jiang, Z. Q. Li, L.-C. Tung, M. E. Schwartz, M. Takita, Y. J. Wang, P. Kim, and H. L. Stormer, Physical Review Letters **104**, 067404 (2010).
[5] A. B. Kuzmenko, Review of Scientific Instruments **76**, 083108 (2005).
[6] M. E. Levinshtein, S. L. Rumyantsev, and M. S. Shur, eds., *Properties of Advanced Semiconductor Materials* (John Wiley and Sons, New York, 2001).
[7] Y. A. Bychkov and G. Martinez, Physical Review B **77**, 125417 (2008).
[8] K. Shizuya, Physical Review B **81**, 075407 (2010).
[9] C. Faugeras, S. Berciaud, P. Leszczynski, Y. Henni, K. Nogajewski, M. Orlita, T. Taniguchi, K. Watanabe, C. Forsythe, P. Kim, R. Jalil, A. K. Geim, D. M. Basko, and M. Potemski, Physical Review Letters **114**, 126804 (2015).
[10] M. A. H. Vozmediano, Nature Physics **7**, 671 (2011).
[11] Z.-G. Chen, Z. Shi, W. Yang, X. Lu, Y. Lai, H. Yan, F. Wang, G. Zhang, and Z. Li, Nature Communications **5**, 4461 (2014).
